# Supplementary material for: Data Splits and Metrics for Method Benchmarking on Surgical Action Triplet Datasets
Source: arXiv:2204.05235 source file (2023-02-28)
Supplement: Supplementary file 1 [file 09-appendix.tex]

\clearpage
\appendix
\counterwithin{table}{section}
\section{Appendix I}
\begin{table}[htp]
\centering
    \setlength{\tabcolsep}{5pt}
    \captionsetup{skip=0pt,singlelinecheck=off,justification=raggedright}
    \caption{Cholec80 to CholecT45 video filename mapping.}
    \label{table:c2c}
    \resizebox{\textwidth}{!}{%
        \begin{tabular}{@{}llrllrll@{}}
        \toprule
        Cholec80  & CholecT45 & \phantom{abc} & Cholec80  & CholecT45 &\phantom{abc} & Cholec80  & CholecT45 \\ 
        \midrule
        7013HD Bin.01-H264-480 & VID01 && 8425HD Bin.01-H264-480 & VID26 && 9066HD Bin.01-H264-480 & VID52 \\ 
        7201HD Bin.01-H264-480 & VID02 && 8554HD Bin.02-H264-480 & VID27 && 9245HD Bin.01-H264-480 & VID56 \\ 
        7301HD Bin.01-H264-480 & VID04 && 8577HD Bin.01-H264-480 & VID29 && 9285HD Bin.01-H264-480 & VID57 \\ 
        7345HD-H264-480	& VID05 && 8611HD Bin.01-H264-480 & VID31 && 9361HD Bin.01-H264-480 & VID60 \\ 
        7348HD Bin.01-H264-480 & VID06 && 8667HD Bin.01-H264-480 & VID32 && 9443HD Bin.01-H264-480 & VID62 \\ 
        7487HD Bin.01-H264-480 & VID08 && 8897HD Bin.01-H264-480 & VID35 && 9544HD Bin.01-H264-480 & VID65 \\ 
        7535HD Bin.01-H264-480 & VID10 && 8906HD Bin.01-H264-480 & VID36 && 9559HD Bin.01-H264-480 & VID66 \\ 
        7695HD Bin.01-H264-480 & VID12 && 9292HD Bin.01-H264-480 & VID40 && 9624HD Bin.01-H264-480 & VID68 \\ 
        7697HD Bin.01-H264-480 & VID13 && 7699HD Bin.01-H264-480 & VID42 && 9674HD Bin.01-H264-480 & VID70 \\ 
        7719HD Bin.01-H264-480 & VID14 && 7947HD Bin.01-H264-480 & VID43 && 9764HD Bin.01-H264-480 & VID73 \\ 
        7754HD Bin.01-H264-480 & VID15 && 8353HD Bin.01-H264-480 & VID47 && 9955HD Bin.01-H264-480 & VID74 \\ 
        7964HD Bin.01-H264-480 & VID18 && 8714HD Bin.01-H264-480 & VID48 && 9966HD Bin.01-H264-480 & VID75 \\ 
        8123HD Bin.01-H264-480 & VID22 && 8823HD Bin.01-H264-480 & VID49 && 10133HD Bin.01-H264-1080 & VID78 \\ 
        8132HD-H264-480 & VID23 && 8852HD Bin.01-H264-480 & VID50 && 10206HD Bin.01-H264-1080	& VID79 \\ 
        8307HD Bin.01-H264-480 & VID25 && 8870HD Bin.01-H264-480 & VID51 && 10241HD Bin.01-H264-1080 & VID80 \\
        \bottomrule
        \end{tabular}
    }
\end{table}
